# Supplementary material for: Phase Space Reconstruction from Accelerator Beam Measurements Using Neural Networks and Differentiable Simulations
Source: arXiv:2209.04505 source file (2023-01-26)
Supplement: Supplementary file 1 [file supp.pdf]

# Supplemental Materials

## I. SYNTHETIC BEAM GENERATION

To test the reconstruction algorithm, we designed a beam that had complex correlations in phase space that would be difficult to characterize by conventional methods and would be possible to observe in real accelerator scenarios. The synthetic beam, generated by the Python package *distgen* [1], started as a Gaussian beam with an RMS beamsize of 2 mm in each dimension, central energy of 10 MeV, $\sigma_{p_x} = 10^{-3}$ MeV/c, $\sigma_{p_y} = 0.02$ MeV/c, and $\sigma_{p_z} = 10^{-6}$ MeV/c. We then modified the distribution via the following steps:

- A linear correlation in horizontal phase space $(x, p_x)$ given by the twiss parameters $\beta = 9$ m, $\alpha = 5$ and a geometric emittance of 2.0 mm-mrad.
- A linear correlation in vertical phase space $(y, p_y)$ given by the twiss parameters $\beta = 9$ m, $\alpha = 0$ and a geometric emittance of 2.0 mm-mrad.
- An added polynomial term in transverse position space $(x, y)$ given by the function $y = -0.005[\mathrm{m}] + 0.75x + 50.0[\mathrm{m}^{-1}]x^2$.
- An added periodic term in vertical phase space $(y, p_y)$ given by the function $p_y = 0.05[\mathrm{MeV/c}]\sin(2\pi y/0.03[\mathrm{m}])$.

## II. MODEL CONSTRUCTION AND TRAINING

We generated proposal distributions by transforming samples drawn from a multi-variate normal distribution into real phase space coordinates. The transformation was defined by a neural network containing 4 hidden layers of 50 neurons each, with a hyperbolic tangent activation functions. The output of the nerual network was then scaled by a fixed factor of $10^{-2}$. This scaling is motivated by the expectation that most beams have phase space coordinates on the order of $10^{-3} - 10^{-2}$ times the base coordinate units ([m] for positional, [rad] for momentum coordinates). The output scaling ensured that the transformation weights of the neural network are closer to unity, improving training via gradient descent as is common in machine learning data analysis. In the work presented here we generate and transport $10^5$ particles for each base distribution, enough to represent most beam features while maintaining reasonable computation complexity and memory requirements. Simulated screen images were generated by using a kernel density estimator with a bandwidth half of the pixel resolution of the simulated screen.

Training and testing data sets were generated by selecting every other sample as a training sample and using the remaining samples for the test set, resulting in both sets having 10 samples. The training data was then batched into sets of 5 samples. Adam gradient descent, implemented by the Python package *PyTorch* [2], was used with snapshot ensembling, implemented by the Python package *TorchEnsemble* [3], to train 5 estimators over 2500 training epochs with a maximum learning rate of $10^{-2}$ and a minimum learning rate of $10^{-4}$. Training was executed over a few minutes on a single Nvidia A100 GPU, provided by the NERSC Perlmutter cluster.

## III. EXPERIMENTAL IMAGE PRE-PROCESSING

To improve data quality from raw experimental imaging of the transverse beam distribution at AWA we took several steps to pre-process the images before conducting model training. For each quadrupole strength 50 images were taken at a repetition rate of 1 Hz. These images were sorted by the corresponding measured bunch charge coming off the photoinjector using an integrated current transformer. We retained 3 images from each quadrupole strength that best matched a target bunch charge of 0.9 nC. We selected a square region of interest centered at the mean beam position in the full set of images and a width of 1000 pixels. Then we subtracted a threshold value from each pixel intensity, clipping at zero, chosen by scaling a value chosen by the triangle thresholding method by 1.1. Next we applied a gaussian smoothing filter with a stadandard deviation of 3 pixels. Finally, to reduce the size of the image we down-sampled the image by a factor of 2 to end up with an 500 x 500 pixel image of the transverse beam distribution.

## IV. IMAGE COMPARISONS

In Figures 1 we demonstrate the accuracy of our reconstruction algorithm when reproducing images included in the training data set and predicting previously unseen images from the test set for the synthetic case.


[1] ColwynGulliford, C. Mayes, G. H. Lusk, and H. Slepicka, Colwyngulliford/distgen: Distgen v0.6.6 (2022).

[2] A. Paszke, S. Gross, F. Massa, A. Lerer, J. Bradbury, G. Chanan, T. Killeen, Z. Lin, N. Gimelshein, L. Antiga, A. Desmaison, A. Kopf, E. Yang, Z. DeVito, M. Raison,

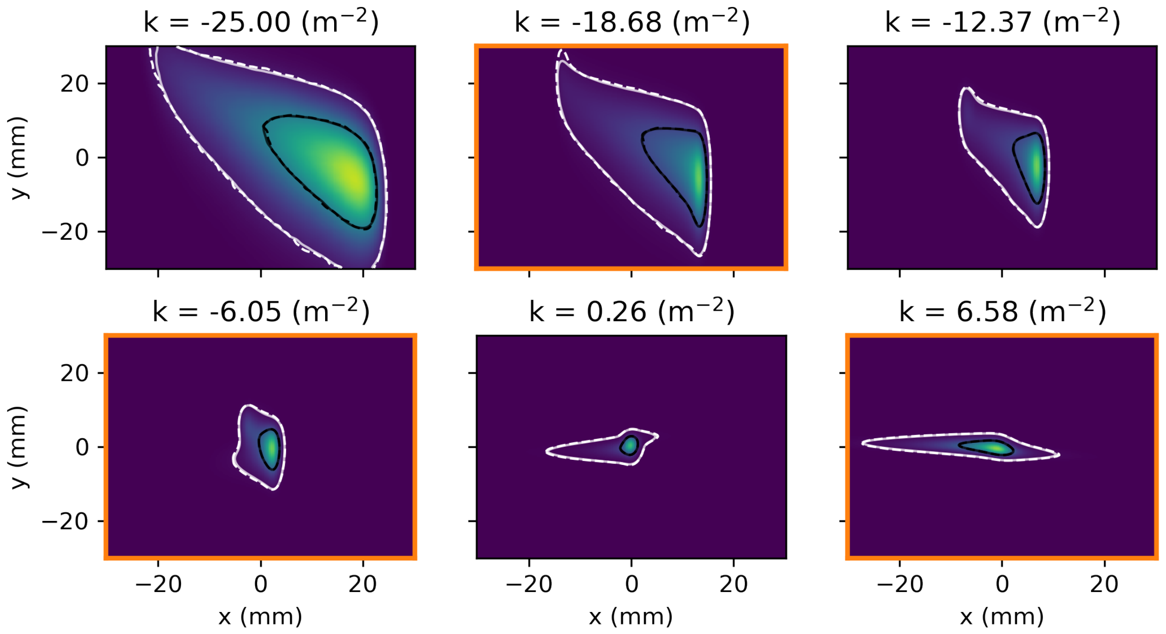


FIG. 1. Comparison of synthetic screen images and reconstructed predictions for a subset of quadrupole strengths. Contours that denote the $50^{th}$ (black) and $95^{th}$ (white) percentiles of the synthetic ground truth (dashed) and reconstructed (solid) distributions. Orange borders denote test samples.


A. Tejani, S. Chilamkurthy, B. Steiner, L. Fang, J. Bai, and S. Chintala, PyTorch: An Imperative Style, High-Performance Deep Learning Library, in *Advances in Neural Information Processing Systems 32*, edited by H. Wallach, H. Larochelle, A. Beygelzimer, F. d. Alché-Buc, E. Fox, and R. Garnett (Curran Associates, Inc., 2019) pp. 8024–8035.

[3] TorchEnsemble-Community/Ensemble-Pytorch (2022), original-date: 2019-09-11T11:44:58Z.
